# Supplementary material for: Linking Surface Facts to Large-Scale Knowledge Graphs
Source: arXiv:2310.14909 source file (2023-10-23)
Supplement: Supplementary file 2 [file app-supp.tex]

\section{Supplementary Materials}
Within the supplementary materials, we release:

\begin{enumerate}
    \item An HTML version of a Jupyter notebook which we use to perform ``qualitative'' evaluation. In the Jupyter notebook, we load the \preranker model (used for the experiments in \S\ref{sec:kg-population}), and perform inference on three randomly sampled instances from the REBEL testing dataset. The purpose of the notebook is to illustrate the inference process with a trained model, as well as the modules necessary to perform the inference. Note that in the camera-ready version we will release all data, resources and trained models.
    \item The testing splits for both REBEL and SynthIE. We release all testing data (see stats in Table~\ref{table:stats}).
    \item The data sample which we used to perform the human study in \S\ref{app:data-quality}.
\end{enumerate}
